# Supplementary material for: Stretchable persistent spin helices in GaAs quantum wells
Source: arXiv:1702.05190 ancillary file (2017-02-20)
Supplement: Supplementary file 1 [file supplementary.pdf.pdf]

Supplementary Information

**Stretchable persistent spin helices in GaAs quantum wells**

Florian Dettwiler,<sup>1</sup> Jiyong Fu,<sup>2,\*</sup> Shawn Mack,<sup>3,†</sup> Pirmin J. Weigele,<sup>1</sup>  
J. Carlos Egues,<sup>2</sup> David D. Awschalom,<sup>3,4</sup> and Dominik M. Zumbühl<sup>1</sup>

<sup>1</sup>*Department of Physics, University of Basel, CH-4056, Basel, Switzerland*

<sup>2</sup>*Instituto de Física de São Carlos,  
Universidade de São Paulo, 13560-970 São Carlos, SP, Brazil*

<sup>3</sup>*California NanoSystems Institute, University of California,  
Santa Barbara, California 93106, USA*

<sup>4</sup>*Institute for Molecular Engineering,  
University of Chicago, Chicago, IL 60637 USA*

---

\* Permanent address: Department of Physics, Qufu Normal University, Qufu, Shandong, 273165, China

† Current address: Naval Research Laboratory, Washington, DC 20375, USA

## I. WAFER STRUCTURE: DETAILS

The quantum well (QW) samples are grown on (001) n-doped substrates, serving as a back gate, with total distance of 1210 nm between back gate and QW, including 600 nm of low-temperature (LT) grown GaAs, see Fig. S1. The LT GaAs creates a barrier by pinning the Fermi level midgap [1]. Thus, in a simple plate capacitor model, the effective distance  $d_B$  between QW and back gate is reduced by the thickness of the LT barrier, increasing

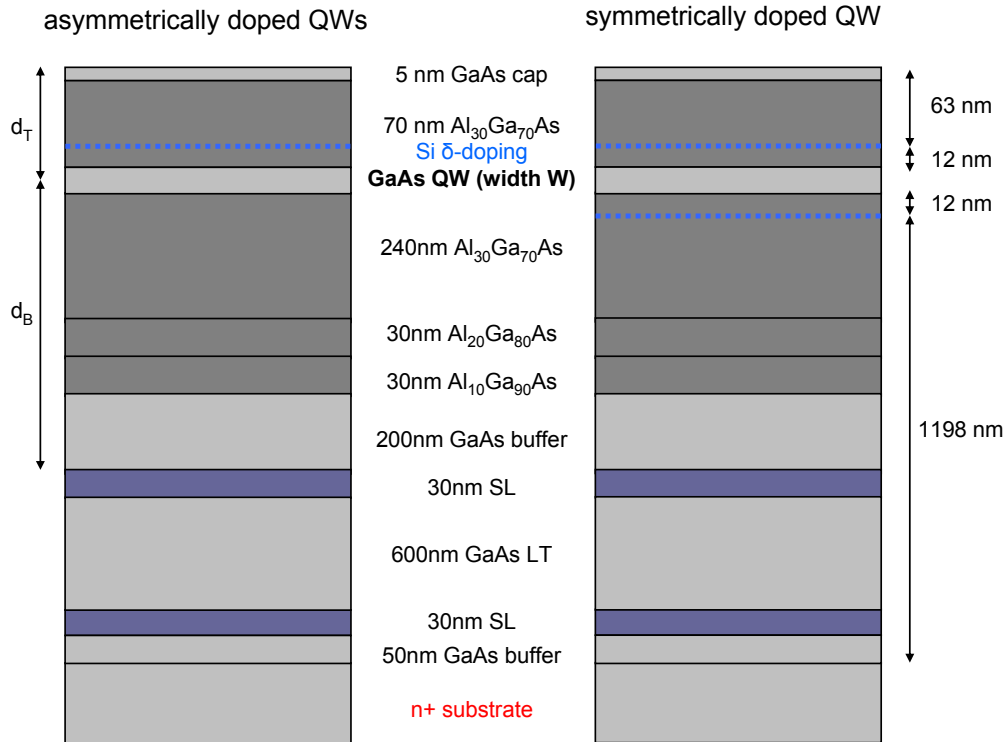

FIG. S1. Quantum well wafer profiles. MBE growth profiles of the asymmetrically (left) and more symmetrically (right) doped QW wafers. The GaAs QW width  $W$  is 8, 9.3, 11 and 13 nm for the asymmetric and 11 nm for the symmetric QW, respectively.

the range of tunability and reducing leakage currents at the same time. Similarly,  $d_T$  is defined as the distance between QW and top gate. Good agreement is found between  $d_{B/T}$  extracted from the measured back/top gate dependence of the carrier density and the as-grown thicknesses of the layers in the QW structure. The QWs are 75 nm below the surface with a setback of 12 nm to the Si  $\delta$ -doping layer above the well for the asymmetric QWs with  $W = 8, 9.3, 11$  and 13 nm and an additional doping layer 12 nm below the 2DEG for

the more symmetric 11 nm QW.

Using top and back gates, the density is tunable typically in a range of  $n \approx 2 - 8 \cdot 10^{11} \text{ cm}^{-2}$  (Fig. S2a) corresponding to mobilities  $\mu \approx 2 - 20 \text{ m}^2/(\text{Vs})$  (Fig. S2b). Tunability is limited by onset of gate leakage and hysteresis issues. For positive  $V_T > 300 \text{ mV}$  and large negative  $V_B < -2 \text{ V}$ , a non-linear gate dependence is observed. Shubnikov-de Haas measurements indicate that all data in this study are in the single 2D subband regime, consistent with the numerical simulations. In section VI we show a more detailed analysis of the Shubnikov-de Haas oscillations. For low densities  $n \lesssim 2 \cdot 10^{11} \text{ cm}^{-2}$ , WAL as a signature of SO coupling becomes very weak or disappears due to the small wave number  $k_F^2 = 2\pi n$ . At even lower densities the electrons become strongly localized by disorder. Hence the lower left corners of Fig. S2a and b corresponding to low densities are not displayed.

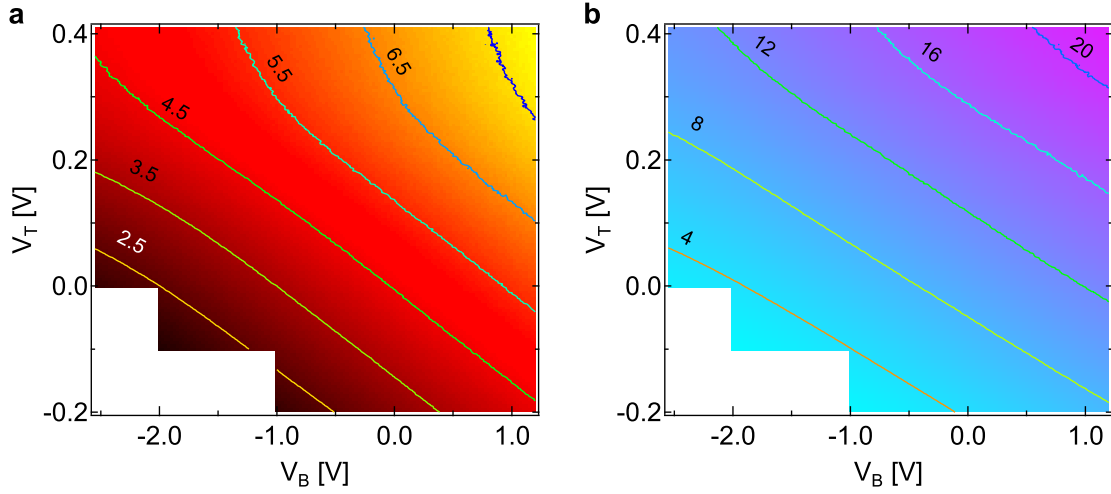

FIG. S2. Density and mobility map of 9.3 nm QW. Charge carrier density  $n$  (a) and mobility  $\mu$  (b) as a function of top gate voltage  $V_T$  and back gate voltage  $V_B$ . Contour lines are labeled in units of  $10^{11} \text{ cm}^{-2}$  (a) and  $\text{m}^2/(\text{Vs})$  (b), respectively. The lower left corner was omitted due to a general lack of WAL at low  $n$ .

## II. TEMPERATURE DEPENDENCE

Elevated temperatures suppress quantum corrections to conductivity, as shown in Fig. S3. The magnetic field position  $B_{\text{SO}}$  of the MC minima, however, appears not affected by temperature (dashed line in Fig. S3), consistent with a spin-orbit (SO) length  $\lambda_{\text{SO}}$  independent of  $T$ . At elevated temperatures, WAL and the  $B_{\text{SO}}$  minima are shallower and eventually can disappear, due to loss of coherence. This leads to a broadening of the WAL-WL-WAL

transition with increasing temperature, i.e. the size of the gate voltage range where WAL is suppressed grows with increasing temperature, see Fig.S4 from left to right. Thus, in absence of symmetry breaking effects of the higher harmonic  $\beta_3$ , the phase coherence defines the width of the WAL-WL-WAL transition in our experiment.

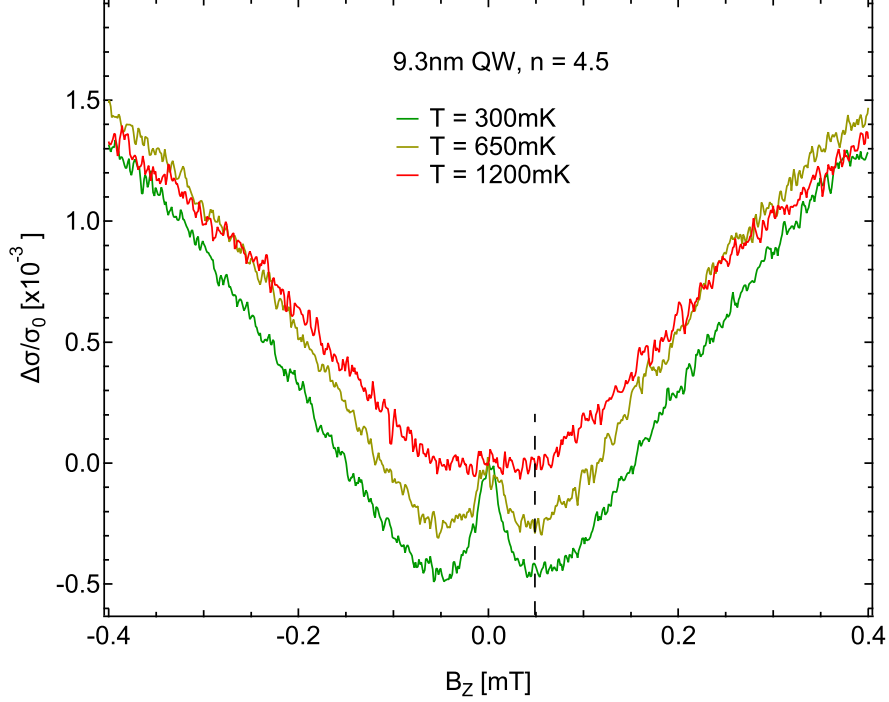

FIG. S3. Temperature dependence of WAL. Magnetoconductance for a specific gate configuration (9.3 nm QW,  $n = 4.5 \cdot 10^{11} \text{ cm}^{-2}$ ,  $V_T = -146 \text{ mV}$ ,  $V_B = 1 \text{ V}$ ) showing clear WAL signature at  $T = 300 \text{ mK}$  (green). The WAL maximum at  $B_Z = 0$  weakens for  $T = 650 \text{ mK}$  (olive), and essentially disappears at  $T = 1200 \text{ mK}$  (red). The position of the MC minima (defined as  $B_{\text{SO}}$ ) appears to be not affected by temperature (dashed vertical line).

### III. NUMERICAL SIMULATIONS

#### A. Self-consistent approach and potential

The confining potential of our GaAs/ $\text{Al}_{0.3}\text{Ga}_{0.7}\text{As}$  wells (see Fig.S5) contains [2]: (i) the structural part  $V_w$  arising from the band offset at the interfaces, (ii) the potential  $V_g$  from the top and back gates, which allows us to adjust the symmetry of the well profile and the electronic densities while keeping the chemical potential  $\mu$  constant, (iii) the doping potential  $V_d$ , which remains fixed at low temperatures (we also use  $V_{g+d} = V_g + V_d$ ), and (iv)

symmetrically doped 11nm QW,  $n=6$

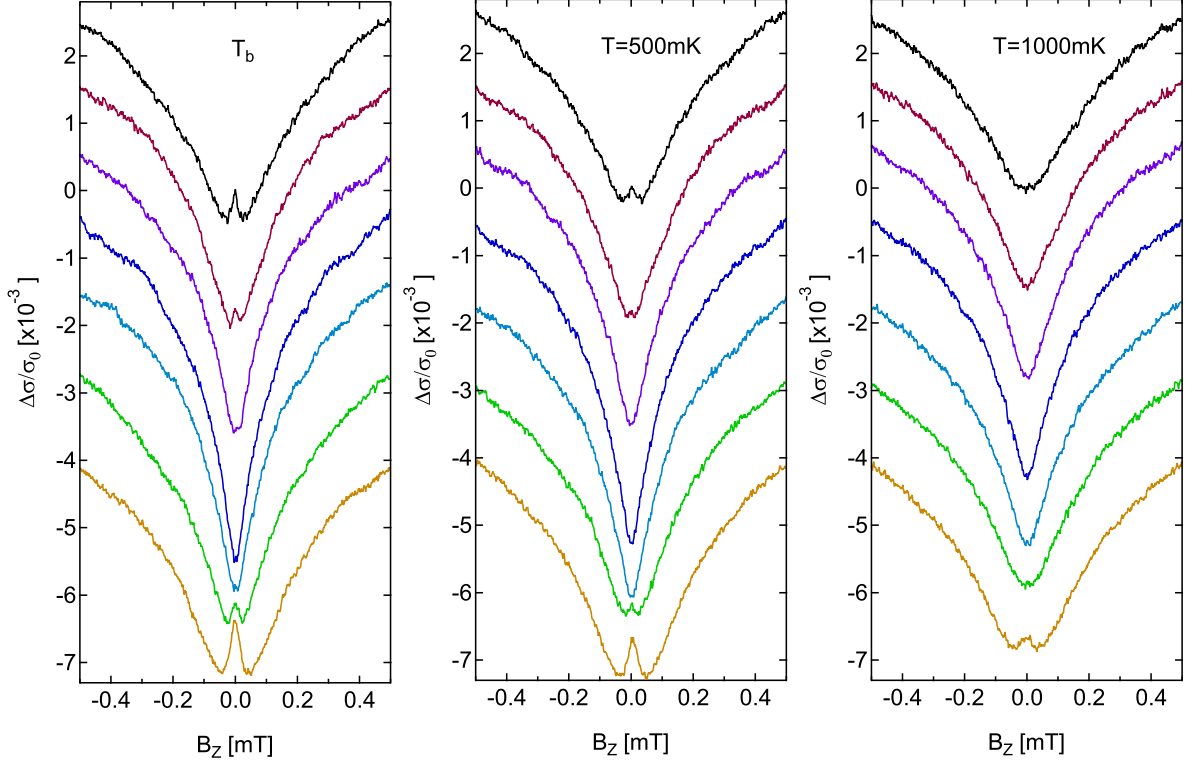

FIG. S4. Temperature dependence of WAL-WL-WAL transition of the more symmetrically doped 11 nm QW, shown for base temperature (left panel), 500 mK (middle panel) and 1 K (right panel) for various  $(V_T, V_B)$  configurations (color coded) at constant density  $n = 6 \cdot 10^{11} \text{ cm}^{-2}$ . The curves are shifted vertically for clarity. Upon increasing  $T$ , WAL weakens and finally disappears on both sides of the low- $T$  symmetry point (see e.g. green and dark brown curve), resulting in a widening of the transition.

the electronic Hartree potential  $V_e$  which depends on carrier density. The 3D electron charge density in the well  $\rho_e$  depends on the total potential  $V_{\text{sc}} = V_w + V_{\text{g+d}} + V_e$ , which in turn depends on  $\rho_e$  via the Hartree term. Hence to find the eigensolutions of the system, we solve the Schrödinger equation for electrons in the total potential  $V_{\text{sc}} = V_w + V_{\text{g+d}} + V_e$ . Both  $V_w$  and  $V_{\text{g+d}}$  depend only on the  $z$  variable (growth direction). Within the Hartree approximation, the electron charge density is  $\rho_e(z, \vec{r}) = 2 \sum_{\nu, \vec{k}} |\varphi_{\nu, \vec{k}}(z, \vec{r})|^2 f_{k, \nu}$ , where  $\varphi_{\nu, \vec{k}}(z, \vec{r}) = \frac{1}{\sqrt{A}} \exp(i\vec{k} \cdot \vec{r}) \psi_{\nu}(z)$  with  $\psi_{\nu}(z)$  being the  $\nu^{\text{th}}$  subband wave function of the well,  $\vec{k}$  the in-plane electron wave vector,  $A$  a normalizing area, and  $f_{k, \nu}$  the Fermi-Dirac distribution. Note that within the Hartree approximation,  $\rho_e(z, \vec{r}) \rightarrow \rho_e(z)$  because of the plane-wave dependence of the wave function in the  $xy$ -plane and hence the Hartree potential  $V_e$  depends only on  $z$ .

Upon summing over  $\vec{k}$ ,  $\rho_e(z)$  simplifies to  $\rho_e(z) = \sum_{\nu} |\psi_{\nu}(z)|^2 n_{\nu}$ , with the electron oc-

cupation of the  $\nu^{\text{th}}$  subband  $n_\nu = \frac{m^*}{\pi \hbar^2} k_B T \ln[1 + \exp(\mu - \mathcal{E}_\nu)/k_B T]$  and confinement energy  $\mathcal{E}_\nu$ . Here  $\mu$  is the electron chemical potential,  $k_B$  the Boltzmann constant and  $T$  the absolute temperature. The areal electron density  $n$  in the well and  $\rho_e(z)$  are related via  $n = \int dz \rho_e(z) = \sum_\nu n_\nu$ . We then solve the resulting one-dimensional Schrödinger equation together with the Poisson's equation for the total charge density  $\rho_{\text{tot}}(z) = \rho_e(z) + \rho_d(z)$ , where  $\rho_d(z)$  denotes the ionized donor concentration profile. We obtain the subband energies  $\mathcal{E}_\nu$  and wave functions  $\psi_\nu(z)$  iteratively within this self consistent procedure when convergence is attained.

The potential profile and the corresponding wave function for the 9.3 nm well based on our self-consistent scheme are shown in Fig. S5 for top and back gates set to  $V_T = 75$  mV and  $V_B = -500$  mV, respectively, corresponding to point 4 in Fig. 2 of the main text.

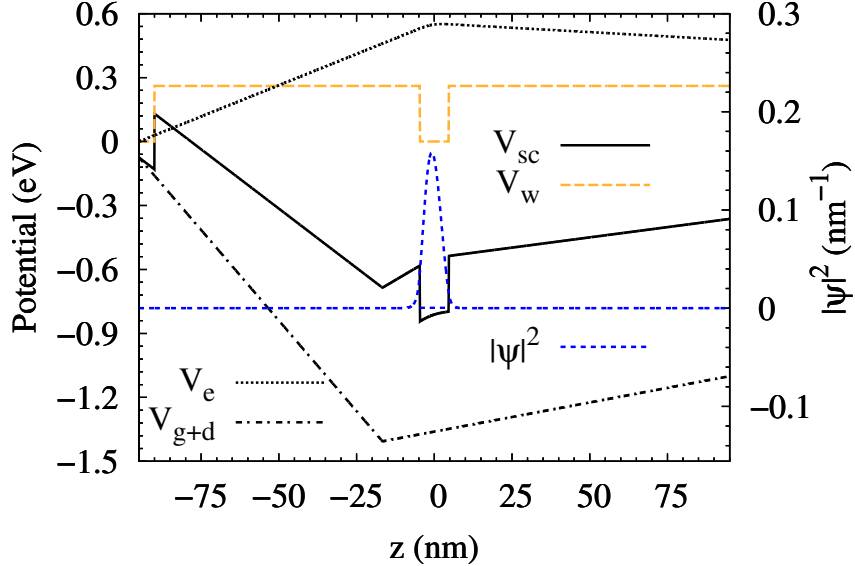

FIG. S5. Self-consistent potential  $V_{\text{sc}}$  and the corresponding wave function  $\Psi$  for our GaAs/ $\text{Al}_{0.3}\text{Ga}_{0.7}\text{As}$  9.3 nm quantum well with the top gate  $V_T = 75$  mV and back gate  $V_B = -500$  mV. The QW band offset potential  $V_w$ , the electron Hartree potential  $V_e$  and the gate plus doping potential  $V_{\text{g+d}}$  are also shown. The first subband energy level is  $\mathcal{E}_1 = -776.0$  meV (indicated by solid green line inside QW), i.e. 16.4 meV below the Fermi energy (not shown), which is pinned at  $-759.6$  meV (i.e., the mid gap energy in bulk GaAs). The resulting carrier density is  $n = 4.5 \cdot 10^{11} \text{ cm}^{-2}$ . Note that the origin of the abscissa is in the center of the well and the wafer surface is located slightly farther away than specified in the growth profile (see also Fig. S1) due to the lever arm measured in the experiment.

## B. Expressions for the SO coupling terms

*Rashba spin-orbit coupling  $\alpha$ .* As shown in Ref. [2], the strength  $\alpha$  of the Rashba coupling can be cast as the expectation value  $\langle \dots \rangle$  of the weighted derivatives of the potential contributions (i)-(iv) above:

$$\alpha = \eta_w \langle \partial_z V_w \rangle + \eta_H \langle \partial_z V_e \rangle + \eta_H \langle \partial_z V_{g+d} \rangle, \quad (\text{S1})$$

with

$$\eta_w = \frac{P^2}{3} \left( \frac{\delta_v/\delta_c}{E_g^2} - \frac{\delta_\Delta/\delta_c}{(E_g + \Delta_w)^2} \right), \quad (\text{S2})$$

and

$$\eta_H = -\frac{P^2}{3} \left( \frac{1}{E_g^2} - \frac{1}{(E_g + \Delta_w)^2} \right), \quad (\text{S3})$$

which involve the bulk quantities of the well layer, such as the band gap  $E_g$  and the usual Kane parameters  $\Delta$  (“spin orbit”) and  $P$ , in addition to the potential offsets  $\delta_i$ ,  $i = c, v, \Delta$  (e.g., in Fig. S5  $V_w = \delta_c[\Theta(W/2 - z) + \Theta(z - W/2)]$  for a well of width  $W$  centered at  $z = 0$ ; here  $\Theta(z)$  is the Heaviside function. See also Fig. S7 and Sec. (III.E) below for a further discussion of these parameters). Even though  $\alpha = \alpha_w + \alpha_e + \alpha_{g+d}$  comprises seemingly independent contributions, we note that each of these  $\alpha_w$ ,  $\alpha_e$ , and  $\alpha_{g+d}$  does depend on all four potentials (i)-(iv) via the self-consistent wave function used in the expectation values. In particular, they all change as we vary the gates (top and back), which allows us to fine tune  $\alpha$  and thus attain the  $\alpha = \beta$  regime when the Dresselhaus term is considered.

We emphasize that the Rashba coefficient  $\alpha$  can be rewritten in terms of an “external” electric field  $E_{\text{ext}} = E_{\text{gate}} + E_d + E_e$ , where we have defined  $E_{\text{gate}} = \frac{1}{e} \langle \partial_z V_g \rangle$ ,  $E_d = \frac{1}{e} \langle \partial_z V_d \rangle$ , and  $E_e = \frac{1}{e} \langle \partial_z V_e \rangle$  with  $e > 0$  the elementary charge. Since the total force on a bound state is zero (Ehrenfest’s theorem), *i.e.*,  $\langle \partial_z V_{sc} \rangle = \langle \partial_z (V_w + V_e + V_g + V_d) \rangle = 0$ , one has the relation of  $\alpha$  with  $E_{\text{ext}}$ ,

$$\alpha = (\eta_H - \eta_w) e E_{\text{ext}}. \quad (\text{S4})$$

Now let us turn to the change of  $\alpha$  due to a variation of  $E_{\text{ext}}$ , *i.e.* a variation  $\delta V_T$  of the top gate voltage and/or a variation  $\delta V_B$  of the back gate voltage, giving  $\delta \alpha = e(\eta_H - \eta_w)(\delta E_{\text{gate}} + \delta E_d + \delta E_e)$ . In our model, the variation  $\delta E_d \simeq 0$  since the doping potential does not vary with the gates. Furthermore, in the case of constant density (as shown in Figs. 2c and 4c of

the main text), we also have  $\delta E_e \simeq 0$  since the rearrangement of the *quantum mechanical* distributions of electrons in the gate range we studied is negligible. Therefore, to keep the carrier density  $n$  unchanged when we tune the gates, we have  $\delta\alpha \simeq e(\eta_H - \eta_w)\delta E_{\text{gate}}$ . Note that in the main text of the paper (and in Figs. 1c and 3c), we use the notation of  $\delta E_z = \delta E_{\text{gate}}$  to describe the change of electric field along the growth direction due to the gates.

*Dresselhaus spin-orbit couplings  $\beta_1$  and  $\beta_3$ .* The linear  $\beta_1$  and cubic  $\beta_3$  coefficients of the Dresselhaus well Hamiltonian arise from the expectation value of the bulk cubic Dresselhaus Hamiltonian [3]. Using our self-consistent electron wave functions, we obtain  $\beta_1 = -\gamma\langle\partial_z^2\rangle$  and  $\beta_3 = \gamma k_F^2/4$ , where  $\gamma$  is the bulk Dresselhaus parameter and  $k_F$  the Fermi wave vector. To a very good approximation the Fermi contours are essentially circles and hence can be approximated by the 2D free electron result  $k_F \simeq \sqrt{2\pi n}$ , with  $n$  being the areal electron density, and  $\beta_3 \simeq \gamma\pi n/2$ .

### C. Input from the experiment

Input for our simulations are mainly based on the experimental conditions:

1. The chemical potential is pinned at mid gap in GaAs ( $= -759.60$  meV) [1].
2. The top gate voltage  $V_T$  and back gate voltage  $V_B$  enter the numerical calculation as boundary conditions when solving the Poisson's equation for  $V_g(z)$ , *i.e.*,  $V_g(-d_T) = -eV_T$  and  $V_g(d_B) = -eV_B$  with the coordinate origin being chosen as the center of the well, which amounts to a linear external gate potential  $V_g(z) = -e\left[V_T + \frac{(V_B - V_T)}{d_B + d_T}(z + d_T)\right]$ . The gate lever arms, *i.e.*, the  $d_T$  and  $d_B$  values, are taken from the experiment and are close to the nominal values from the wafer growth profile.
3. We model the delta-doping regions in our samples by considering monolayer-thick doped regions with an effective ionized areal doping density  $\rho^{\text{eff}}$  used in the simulation, distinct from the nominal doping  $\rho^{\text{nom}}$  specified in the MBE growth.

In the asymmetrically doped wafers, the effective doping density  $\rho^{\text{eff}}$  is chosen so that the areal electron density  $n(V_T, V_B)$  in the QW matches the measured values for all gate voltages using the experimentally determined gate lever arms. We find a donor ionization efficiency

$\rho^{\text{eff}}/\rho^{\text{nom}}$  of about 50% for all asymmetric wafers. We need to introduce the effective doping density  $\rho^{\text{eff}}$  because the simulation does not include effects such as partial absorption of donor electrons e.g. by positive background doping or DX centers, resulting in partial ( $\sim 50\%$ ) rather than full ionization of donors.

In the more symmetrically doped wafer, in contrast to the asymmetric ones, we have two  $\delta$ -doping layers: an upper layer above the QW with effective doping  $\rho_{\text{u}}^{\text{eff}}$  and a lower layer below the QW with effective doping  $\rho_{\text{l}}^{\text{eff}}$ . The effective doping asymmetry ratio  $r = \rho_{\text{l}}^{\text{eff}}/\rho_{\text{u}}^{\text{eff}}$  modifies the Rashba coefficient  $\alpha$  by changing the electric field across the QW. In the experiment, we detect the  $\alpha = \beta$  regime (absence of WAL), where  $\beta \propto \gamma$ . Thus,  $r$  and with it the simulated  $\alpha$  will directly affect the extracted  $\gamma$ . There is no reason to have a  $\gamma$  for the symmetrically doped QW that is different from the asymmetrically doped, but otherwise identical QW. Thus, we choose the doping asymmetry  $r$  by requiring that the Dresselhaus parameter  $\gamma$  take on the same value  $\gamma = 11.6 \text{ eV}\text{\AA}^3$  as for all the asymmetric wafers, while choosing  $\rho_{\text{u}}^{\text{eff}}$  to maintain the measured charge density in the QW. Here, we obtain  $\rho_{\text{u}}^{\text{eff}} \sim 0.61 \cdot \rho_{\text{u}}^{\text{nom}}$  and  $r \sim 0.3$ , i.e., about three times more doping from above than from below the QW.

We note that the QW electron density  $n$  is significantly smaller than the total effective ionized doping  $\rho^{\text{eff}} = \rho_{\text{u}}^{\text{eff}} + \rho_{\text{l}}^{\text{eff}}$ , e.g.  $n \sim 5 \cdot 10^{11} \text{ cm}^{-2}$  versus  $\rho^{\text{eff}} \sim 15 \cdot 10^{11} \text{ cm}^{-2}$ . Due to the close proximity of the QW to the surface and to the interface with the LT GaAs barrier, a large fraction of the ionized donor electrons will populate surface and interface states, rather than the QW. This results in strong band bending at the surface and LT interface, lowering the QW energy below the chemical potential and allowing populate the QW with electrons.

#### D. Fit of the Dresselhaus parameter $\gamma$

With our self-consistent calculation of  $\alpha$  and  $\langle k_z^2 \rangle$  we can determine a so-called  $\gamma$ -map, which gives contours in the  $V_B$  and  $V_T$  space where the condition  $\alpha = \gamma(\langle k_z^2 \rangle - \frac{1}{4}k_F^2)$  is fulfilled. We fit our symmetry points (where  $\alpha \approx \beta$ ) to this map and extract an effective value of  $\gamma = 11.6 \text{ eV}\text{\AA}^3$ . In Fig. S6 we show our experimentally determined symmetry points and the fit to these, as well as contours with similar values for  $\gamma$ . Our extracted value of  $\gamma$  is clearly in good agreement with the data, since the other values of  $\gamma$  would require symmetry points at different values of  $V_B$  and  $V_T$ .

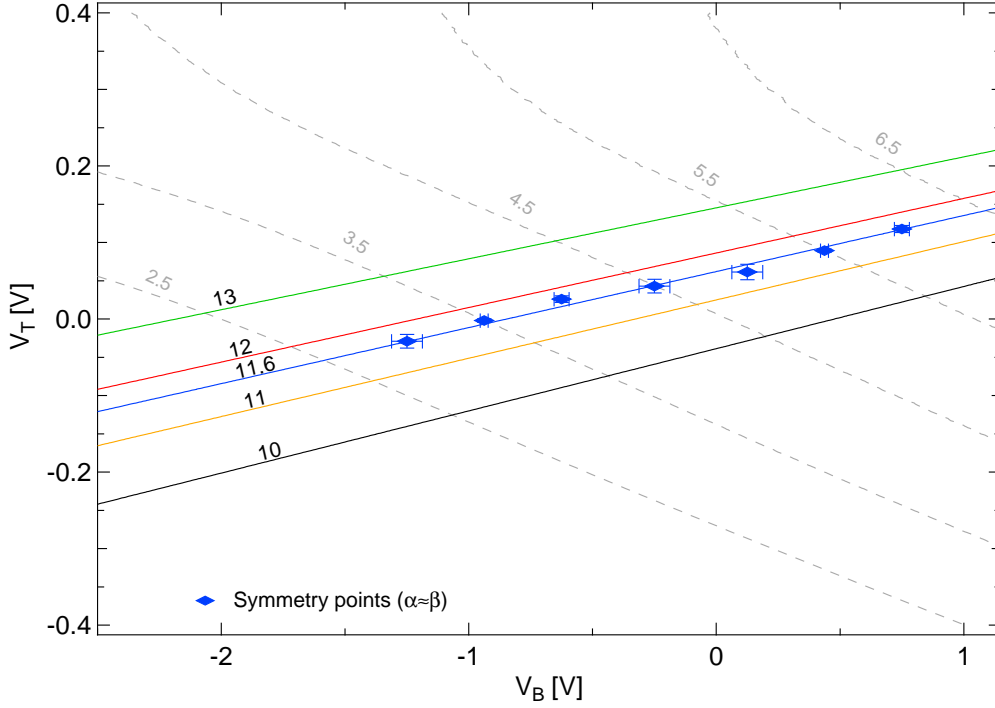

FIG. S6.  **$\gamma$ -map.** Contours of various values for  $\gamma$  for the 9.3nm wafer and the determined symmetry points with their fit. The value of  $\gamma$  is indicated at each contour in units of  $\text{eV}\text{\AA}^3$

### E. Gate voltages and contours of constant density

We will now describe the effect of the gate voltages within a quantum mechanical model and compare the results to that of a simple classical plate capacitor model.

*Quantum mechanical description.* Here we treat the variation  $\delta V_g^T(z)$  due to a change of top gate voltage  $\delta V_T$  and the variation  $\delta V_g^B(z)$  due to a change of back gate voltage  $\delta V_B$  as a perturbation and obtain the first order correction to the lowest subband energy,  $\delta \mathcal{E}_1 = \delta \mathcal{E}_1^T + \delta \mathcal{E}_1^B$  with

$$\delta \mathcal{E}_1^T = \langle \psi^0 | \delta V_g^T(z) | \psi^0 \rangle = -e \frac{d_B - \langle \psi^0 | z | \psi^0 \rangle}{d_B + d_T} \delta V_T, \quad (\text{S5})$$

and

$$\delta \mathcal{E}_1^B = \langle \psi^0 | \delta V_g^B(z) | \psi^0 \rangle = -e \frac{d_T + \langle \psi^0 | z | \psi^0 \rangle}{d_B + d_T} \delta V_B, \quad (\text{S6})$$

where  $\psi^0$  is the envelope function in absence of  $\delta V_g^T(z)$  and  $\delta V_g^B(z)$ , and  $d_T$  ( $d_B$ ) the top (back) gate lever arms. Notice that in all our wafers the well width  $W \ll d_T(d_B)$ , which

ensures  $\langle \psi^0 | z | \psi^0 \rangle \ll d_T(d_B)$  since  $\psi^0$  is mostly confined in the well (if  $\psi^0$  is symmetric with respect to the center of the well, i.e., in a symmetric wafer,  $\langle \psi^0 | z | \psi^0 \rangle$  is always zero). Therefore we have

$$\delta \mathcal{E}_1^T \simeq -e \frac{d_B}{d_B + d_T} \delta V_T, \quad \delta \mathcal{E}_1^B \simeq -e \frac{d_T}{d_B + d_T} \delta V_B. \quad (\text{S7})$$

The resulting change of carrier density  $\delta n$  can be straightforwardly written as

$$\delta n = -\frac{m^*}{\pi \hbar^2} (\delta \mathcal{E}_1^T + \delta \mathcal{E}_1^B) = \frac{m^*}{\pi \hbar^2} e \left( \frac{d_B}{d_B + d_T} \delta V_T + \frac{d_T}{d_B + d_T} \delta V_B \right). \quad (\text{S8})$$

Note that this change of density considers only the response to changes of the gate voltages and neglects the resulting change of the self-consistent Hartree potential. When the self-consistent Hartree potential is also included, the resulting gate lever arm is identical to the lever arm obtained in the plate capacitor model (see below) and reproduces the experimentally measured density changes very well. On a contour of constant density, the Hartree potential is essentially constant in the voltage range considered here, and thus drops out. From Eq. S8, a constant density results for  $\delta V_T/d_T = -\delta V_B/d_B$ . Furthermore, the change of electric field for constant density is

$$\delta E_z = \frac{\delta V_T - \delta V_B}{d_T + d_B} = \frac{\delta V_T + \delta V_T \frac{d_B}{d_T}}{d_T + d_B} = \frac{\delta V_T}{d_T} \frac{d_T + d_B}{d_T + d_B} = \frac{\delta V_T}{d_T} = -\frac{\delta V_B}{d_B}. \quad (\text{S9})$$

*Classical plate capacitor model.* Based on a simple plate capacitor model, a variation of top gate  $\delta V_T$  and back gate  $\delta V_B$  induces a change of carrier density  $\delta n^T$  and  $\delta n^B$ , respectively,

$$\delta n^T = \frac{\epsilon \epsilon_0}{e} \frac{\delta V_T}{d_T}, \quad \delta n^B = \frac{\epsilon \epsilon_0}{e} \frac{\delta V_B}{d_B}, \quad (\text{S10})$$

which also agrees very well with the measured gate effect. To ensure a constant density when varying the top and back gates, i.e.,  $\delta n^T + \delta n^B = 0$ , we obtain,  $\delta V_T/d_T = -\delta V_B/d_B$ , identical to the expression from the quantum mechanical description. Furthermore, the change of average electric field on the left and right of the 2DEG plate is  $\delta E_z = 1/2(\delta V_T/d_T - \delta V_B/d_B)$ . On a contour of constant density, this again becomes  $\delta E_z = \delta V_T/d_T = -\delta V_B/d_B$ , as before in the quantum description. For simplicity, we use  $\delta E_z = 1/2(V_T/d_T - V_B/d_B)$ , i.e. using the actual applied gate voltages, rather than only changes of voltages, as a practical choice

of the origin of  $E_z$ , e.g. for Figs. 2c and 4c (main text).

#### F. Estimate of the error bars in the Rashba coupling due to the uncertainties in input parameters

The Rashba coupling strength  $\alpha$  is more sensitive to the band parameters, especially to the band offsets of the quantum well (see expression for  $\alpha$  above), than the Dresselhaus  $\beta_1$ , which in our phenomenological description solely depends on the well confinement via the wave function. Therefore, to extract a reliable  $\gamma$  based on the condition  $\alpha = \beta$  (locked  $\alpha = \beta$  regime or absence of WAL), it is essential to assess how sensitive the Rashba coupling is to the band parameters.

A sketch of the conduction and valence-band offsets for our GaAs/Al<sub>0.3</sub>Ga<sub>0.7</sub>As quantum well is shown in Fig. S7, where the relevant bulk parameters are indicated. The commonly accepted band gap in GaAs at low temperature is 1.519 eV [4–8], and the band gap in Al<sub>0.3</sub>Ga<sub>0.7</sub>As is  $1.951 \pm 0.006$  eV [5]. The main offsets of a GaAs/Al<sub>0.3</sub>Ga<sub>0.7</sub>As quantum well,  $\delta_c$  (electrons) and  $\delta_v$  (heavy and light holes), are taken from literature with uncertainties of about 2% [5]. We obtain the split-off hole offset  $\delta_\Delta$  straightforwardly through the relation,  $\delta_\Delta = \delta_v + \Delta_b - \Delta_w$  with  $\Delta_w$  ( $\Delta_b$ ) the split-off gap in the well (barrier), see Fig. S7 and Table I. The split-off gap  $\Delta_b$  of the barrier is obtained from linear interpolation of the GaAs and AlAs values [6]. From the uncertainties in  $\delta_v$ ,  $\Delta_b$  and  $\Delta_w$ , one can evaluate the error bar of  $\delta_\Delta$  [9].

Another crucial quantity determining the Rashba  $\alpha$  is the Kane parameter  $P$  (see Eq. 1-3), usually expressed via the quantity  $E_P = 2m_0P^2/\hbar^2$  (see e.g. Ref. [6]), with  $m_0$  the bare electron mass. We take  $E_P$  for GaAs from the widely accepted values quoted by Hermann and Weisbuch [10] (see also [6]), who extracted this parameter via a detailed fitting procedure involving both the effective mass and the  $g$  factor. In their fitting, an error of effective mass and  $g$  factor less than 1% has been assumed. As pointed out by Vurgaftman *et al.* in their classic review Ref. [6], other estimates of  $E_P$  with smaller errors seem to have internal inconsistencies. The band parameters and Kane parameter  $E_P$  used in the simulations and their corresponding errors are summarized in Table I.

With all these parameters and the corresponding errors at hand, we can now evaluate the Rashba coefficient  $\alpha$  and its uncertainty. The  $\alpha$  coefficient for our 9.3 nm well as a function

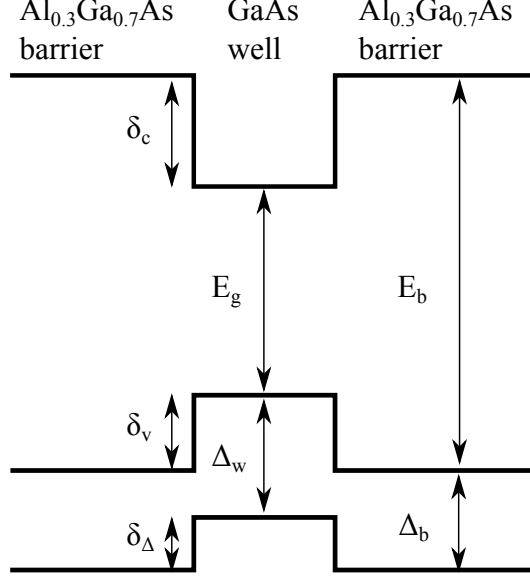

FIG. S7. Schematic of the band offsets for GaAs/AlGaAs well.  $E_g$  ( $E_b$ ) and  $\Delta_w$  ( $\Delta_b$ ) are the fundamental band gap and the split-off gap in the well (barrier), respectively.  $\delta_i$  ( $i = c, v, \Delta$ ) denote the corresponding band offsets:  $\delta_c$  for conduction band,  $\delta_v$  for heavy hole (and light hole), and  $\delta_\Delta$  for split-off hole.

TABLE I. Main relevant parameters for the Rashba coupling. The unit is in eV

|       | $\Delta_b(\text{AlAs})$                  | $\Delta_w(\text{GaAs})$                    | $\Delta_b(\text{Al}_{0.3}\text{Ga}_{0.7}\text{As})$ |
|-------|------------------------------------------|--------------------------------------------|-----------------------------------------------------|
| Value | 0.30 <sup>a,e</sup> (0.28 <sup>c</sup> ) | 0.341 <sup>a-f</sup> (0.340 <sup>h</sup> ) | 0.329 <sup>c</sup>                                  |
| Error | 0.02 (6.7%)                              | 0.001 (0.3%)                               | 0.007 (2%)                                          |

|       | $\delta_c$                | $\delta_v$                | $\delta_\Delta$          | $E_P$                     |
|-------|---------------------------|---------------------------|--------------------------|---------------------------|
| Value | 0.261 <sup>b</sup>        | 0.171 <sup>b</sup>        | 0.159 <sup>f</sup>       | 28.9 <sup>c,g</sup>       |
| Error | 0.003 (1.2%) <sup>b</sup> | 0.003 (1.8%) <sup>b</sup> | 0.01 (6.3%) <sup>f</sup> | 0.9 (3.1%) <sup>c,g</sup> |

<sup>a</sup>Ref. [4], <sup>b</sup>Ref. [5], <sup>c</sup>Ref. [6], <sup>d</sup>Ref. [7], <sup>e</sup>Ref. [8], <sup>f</sup>Ref. [9], <sup>g</sup>Ref. [10], and <sup>h</sup>Ref. [11].

of back gate is shown in Fig. S8, where we vary both the top and back gates so that the curve follows a constant density,  $n = 4.5 \cdot 10^{11} \text{ cm}^{-2}$ . The  $\alpha$  plotted here actually corresponds to the one shown in Fig. 2c (red solid curve) of the paper. The error bar of  $\alpha$  for several values of the back gate is also shown in Fig. S8.

The resulting error of  $\alpha$  is found to be  $\sim 8\%$ , with two dominating contributions,  $\sim 4\%$  from the uncertainty of the band parameters and  $\sim 3\%$  from the Kane parameter  $P$ . The remaining  $\sim 1\%$  error of  $\alpha$  arises from the uncertainty of the measured carrier density, the effective lever arms, and the resulting uncertainty of the doping efficiency ( $\rho^{\text{eff}}/\rho^{\text{nom}}$ ). This error analysis holds for all wafers used in this study. Note that to determine  $\gamma$  (Fig. 2c),

we use the error bars arising from experimental uncertainty ( $1 - 2\%$ ) only, not taking into account the 13 nm wafer data due to its significantly larger error bar (using three data points from the 8, 9.3 and 11 nm wafers in Fig. 2c). We then add the larger systematic error, resulting in a total error on  $\gamma$  of about  $9 - 10\%$  or  $\pm 1 \text{ eV}\text{\AA}^3$ . Finally, we note that the  $\gamma$  extracted from the 13 nm wafer is also consistent with this  $\gamma$ -value.

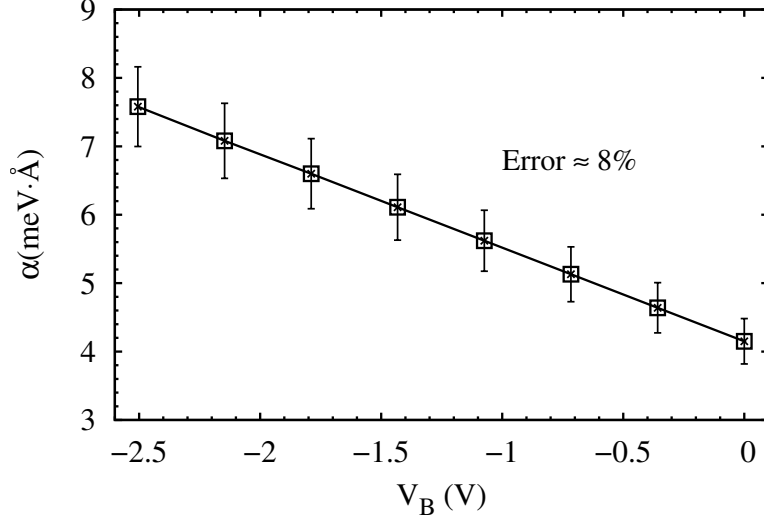

FIG. S8. Error bar on the calculated Rashba coefficient  $\alpha$ . Rashba coupling strength  $\alpha$  as a function of  $V_B$  on a contour of constant density  $n = 4.5 \cdot 10^{11} \text{ cm}^{-2}$  for the 9.3 nm QW and corresponds to the  $\alpha$  curve (the red solid curve) in Fig. 1c. The error bar due to the uncertainty in input parameters for several values of back gate is also shown. The error is about 8%.

#### IV. EFFECTIVE SPIN-ORBIT MAGNETIC FIELD

For a 001-grown GaAs well, the linear-in-the-wave-vector SO term contains both the Rashba and Dresselhaus contributions

$$H_{\text{SO}}^{(1)} = \alpha(k_x\sigma_y - k_y\sigma_x) + \beta_1(k_y\sigma_y - k_x\sigma_x), \quad (\text{S11})$$

with  $\alpha$  and  $\beta_1 = \gamma\langle k_z^2 \rangle$  the linear Rashba and (“bare”) Dresselhaus coefficients, respectively, and  $k_{x,y}$  the electron wave vector along the  $\hat{x}||[100]$  and  $\hat{y}||[010]$  directions. The cubic (in  $k$ ) Dresselhaus term reads

$$H_{\text{SO}}^{(3)} = \gamma(k_x k_y^2 \sigma_x - k_y k_x^2 \sigma_y). \quad (\text{S12})$$

Equations S11 and S12 can be rewritten in terms of sin/cos functions of  $\phi$  (1st harmonic) and  $3\phi$  (3rd harmonic) with  $\phi$  the polar angle between  $\mathbf{k}$  and  $x$  axis. The linear term has only the first harmonic contribution

$$H_{\text{SO}}^{(1)} = k\{[\alpha \cos(\phi) + \beta_1 \sin(\phi)]\sigma_y - [\alpha \sin(\phi) + \beta_1 \cos(\phi)]\sigma_x\}, \quad (\text{S13})$$

while the cubic term contributes to both the first and third harmonics,

$$H_{\text{SO}}^{(3)} = k\{\beta_3[\cos(\phi) - \cos(3\phi)]\sigma_x - \beta_3[\sin(\phi) + \sin(3\phi)]\sigma_y\}, \quad (\text{S14})$$

with  $\beta_3 = \gamma k^2/4$  the cubic Dresselhaus coefficient.

*Rotating the reference frame.* For convenience, we further rewrite the above equations in the rotated coordinate system. The  $\hat{x}_+||[110]$  and  $\hat{x}_-||[\bar{1}10]$ . The linear SO term becomes

$$\begin{aligned} \mathcal{H}_{\text{SO}}^{(1)} &= (-\alpha + \beta_1)k_- \sigma_+ + (\alpha + \beta_1)k_+ \sigma_- \\ &= k[(-\alpha + \beta_1) \sin(\theta) \sigma_+ + (\alpha + \beta_1) \cos(\theta) \sigma_-], \end{aligned} \quad (\text{S15})$$

while the cubic term reads

$$\begin{aligned} \mathcal{H}_{\text{SO}}^{(3)} &= \frac{\gamma}{2}(k_+^2 - k_-^2)(k_- \sigma_+ - k_+ \sigma_-) \\ &= k\{\beta_3[\sin(3\theta) - \sin(\theta)]\sigma_+ - \beta_3[\cos(3\theta) + \cos(\theta)]\sigma_-\}, \end{aligned} \quad (\text{S16})$$

with  $\theta$  the polar angle in the rotated coordinate system, i.e., the angle between  $\mathbf{k}$  and  $x_+$  axis. From Eqs. S15 and S16, one has all the first- and third-harmonic terms,

$$\begin{aligned} \mathcal{H}_{\text{SO}} &= \mathcal{H}_{\text{SO}}^{(1)} + \mathcal{H}_{\text{SO}}^{(3)} \\ &= k\{[(-\alpha + \beta) \sin(\theta) + \beta_3 \sin(3\theta)]\sigma_+ + [(\alpha + \beta) \cos(\theta) - \beta_3 \cos(3\theta)]\sigma_-\}, \end{aligned} \quad (\text{S17})$$

with  $\beta = \beta_1 - \beta_3$  the renormalized “linear” Dresselhaus coefficient. Note that here  $\beta = \beta_1 - \beta_3$  implying that part of the cubic Dresselhaus term ( $\mathcal{H}_{\text{SO}}^{(3)}$ ) renormalizes the linear parameter  $\beta_1$  thus altering the condition for attaining the regime of matched SO strength (or absence of WAL) from  $\alpha = \beta_1$  to  $\alpha = \beta$ . With the approximation (main text)  $\beta_3 \simeq \gamma \pi n/2$ , which neglect the small anisotropy of the Fermi wave vector, this renormalization renders the Dresselhaus coupling  $\beta$  density dependent thus providing a means to gate-tune  $\beta$  and

attain the “dynamical” locking  $\alpha = \beta$  over a wide range of gate voltages, as described in the main text (see Fig. 2b). The remaining part of the cubic term (third harmonic) breaks the angular symmetry of the SO terms and is detrimental to the protection from relaxation.

*Effective SO magnetic fields.* It is convenient to reexpress the spin-orbit Hamiltonian  $\mathcal{H}_{\text{SO}}$  in a compact form, i.e, in terms of an effective magnetic field  $\mathbf{B}_{\text{RD}}(\mathbf{k})$  due to the Rashba and Dresselhaus terms,

$$\mathcal{H}_{\text{SO}} = \frac{1}{2}g\mu_B\mathbf{B}_{\text{RD}}(\mathbf{k}) \cdot \boldsymbol{\sigma}, \quad (\text{S18})$$

with  $g$  the electron g-factor in the well,  $\mu_B$  the Bohr magneton and

$$\mathbf{B}_{\text{RD}}(\mathbf{k}) = \mathbf{B}_{\text{RD}}^{(1)}(\mathbf{k}) + \mathbf{B}_{\text{RD}}^{(3)}(\mathbf{k}), \quad (\text{S19})$$

$$\mathbf{B}_{\text{RD}}^{(1)}(\mathbf{k}) = \frac{2}{g\mu_B}k [(-\alpha + \beta)\sin(\theta)\hat{x}_+ + (\alpha + \beta)\cos(\theta)\hat{x}_-], \quad (\text{S20})$$

and

$$\mathbf{B}_{\text{RD}}^{(3)}(\mathbf{k}) = \frac{2}{g\mu_B}k [\beta_3\sin(3\theta)\hat{x}_+ - \beta_3\cos(3\theta)\hat{x}_-], \quad (\text{S21})$$

where  $\mathbf{B}_{\text{RD}}^{(1)}(\mathbf{k})$  and  $\mathbf{B}_{\text{RD}}^{(3)}(\mathbf{k})$  are the first- and third-harmonic SO fields, respectively. [12, 13] Note that within the approximation  $\beta_3 \simeq \gamma\pi n/2$  both  $\mathbf{B}_{\text{RD}}^{(1)}(\mathbf{k})$  and  $\mathbf{B}_{\text{RD}}^{(3)}(\mathbf{k})$  are linear in  $k$ . In addition, observe that for matched SO couplings  $\alpha = \pm\beta$ ,  $\mathbf{B}_{\text{RD}}^{(1)}(\mathbf{k})$  is unidirectional, i.e., its direction in real space is  $k$  independent, while  $\mathbf{B}_{\text{RD}}^{(3)}(\mathbf{k})$  has a  $k$ -dependent direction (through  $3\theta$ ), as can be seen in Eqs. (S20) and (S21), respectively. As discussed in the main text, the third harmonic contribution of the cubic Dresselhaus term is detrimental to spin protection because its resulting effective field  $\mathbf{B}_{\text{RD}}^{(3)}(\mathbf{k})$  causes random spin precessions upon momentum scattering even at  $\alpha = \pm\beta$ .

## V. DIFFUSIVE SPIN-ORBIT TIME AND LENGTH

Here we calculate several relevant time and length scales in our systems by using a simple 2D diffusive model.

### A. Random walk in two dimensions: diffusive motion

We determine the theoretical spin relaxation time  $\tau_{\text{eff}}$  via the D'Yakonov-Perel' (DP) spin dephasing mechanism: as an electron performs a two-dimensional random walk in real space due to momentum scattering, it precesses about the momentum-dependent spin-orbit field  $\mathbf{B}_{\text{RD}}(\mathbf{k})$ , whose direction is randomly changing as well, thus accruing random precessional phases and spin dephasing after many scattering events in a time  $\tau_{\text{DP}}$ .

Let  $r_{x_i} = \sum_{j=1}^N \delta_{x_i}^j$  be the  $x_i$  component of the electron position vector on the  $(x_-, x_+)$  plane after a total of  $N$  scattering events whose  $j$ th displacement along the corresponding direction we denote by  $\delta_{x_i}^j$ . As usual in random walks [14],  $\langle r_{x_i} \rangle_t = 0 = \langle \delta_{x_i}^j \rangle_t$  and its variance  $\sigma_{x_i}^2 = \langle r_{x_i}^2 \rangle_t = N \langle (\delta_{x_i}^j)^2 \rangle_t$ . Here  $\langle \dots \rangle_t$  denotes a time average over the survival probability  $P(t) = \exp(-t/\tau_p)$ , with  $\tau_p$  being the momentum scattering time. Here,  $P(t)$  is the probability of surviving a time  $t$  without suffering a collision (momentum scattering). The individual mean square displacement  $\langle (\delta_{x_i}^j)^2 \rangle_t = \langle (v_{x_i} t)^2 \rangle_t$  is independent of  $j$  and equals to  $\langle (\delta_{x_i}^j)^2 \rangle_t = v_F^2 \tau_p^2$ , where we have used  $\langle v_{x_i}^2 \rangle_t = v_F^2/2$  and  $\langle t^2 \rangle_t = 2\tau_p^2$ . Since  $N = \tau_{\text{DP}}/\tau_p$ , we find  $\sigma_{x_i}^2 = (\tau_{\text{DP}}/\tau_p) v_F^2 \tau_p^2 = \tau_{\text{DP}} l^2/\tau_p = 2D\tau_{\text{DP}}$ , where  $l = v_F \tau_p$  is the electron mean free path and  $D = l^2/2\tau_p$ . We now define the spin diffusion lengths along  $x_+$  and  $x_-$  via  $\lambda_{\text{DP},x_+}^2 = \sigma_{x_+}^2 = 2D\tau_{\text{DP}}$  and  $\lambda_{\text{DP},x_-}^2 = \sigma_{x_-}^2 = 2D\tau_{\text{DP}}$ , respectively. Since  $\lambda_{\text{DP},x_+} = \lambda_{\text{DP},x_-} = \lambda_{\text{DP}}$ , the direction of the diffusion is isotropic and the product  $\lambda_{\text{DP},x_+} \lambda_{\text{DP},x_-} = \lambda_{\text{DP}}^2 = 2D\tau_{\text{DP}}$  gives the characteristic loop area  $A$  of a closed trajectory. Thus we obtain  $\lambda_{\text{DP}} = \sqrt{2D\tau_{\text{DP}}}$  for the conversion between spin relaxation time and spin diffusion length. As already shown in the main text and methods, using an Aharonov-Bohm phase of  $\Delta\varphi = 1$  from the flux through  $A$ , we can convert the experimental  $B_{\text{SO}}$  to a SO length  $\lambda_{\text{SO}} = \sqrt{\hbar/2eB_{\text{SO}}}$ , which we can further convert to a SO time  $\tau_{\text{SO}} = \lambda_{\text{SO}}^2/(2D)$ .

For a degenerate 2DEG, the individual DP spin relaxation rates are spin-direction dependent, with  $\tau_{\text{DP},s_{x_i}}$  ( $i = +, -, z$ ) for spins polarized along  $\hat{x}_+$ ,  $\hat{x}_-$ , and  $\hat{z}$ , being described by [15]

$$\frac{1}{\tau_{\text{DP},s_{x_{\pm}}}} = \frac{2\tau_1 k_F^2}{\hbar^2} \left[ (\alpha \pm \beta)^2 + \frac{\tau_3}{\tau_1} \beta_3^2 \right], \quad (\text{S22})$$

$$\frac{1}{\tau_{\text{DP},s_z}} = \frac{4\tau_1 k_F^2}{\hbar^2} \left[ \alpha^2 + \beta^2 + \frac{\tau_3}{\tau_1} \beta_3^2 \right]. \quad (\text{S23})$$

Here,  $\tau_1$  is the transport scattering time  $\tau_p$  and we assume  $\tau_1 \geq \tau_3$ , where  $\tau_3$  is the third moment of the momentum relaxation time [15]. For dominant small angle scattering, one

obtains  $\tau_1 = 9\tau_3$ .

## B. Effective spin-dephasing time and effective spin-diffusion length

Note that Eqs. S22 and S23 describe the relaxation of polarized spins, e.g. optically excited spins. In contrast, there is a negligible spin polarization in our transport experiment, therefore we define an effective  $\tau_{\text{eff}}$  for a random spin, by taking the average of the spin lifetimes

$$\tau_{\text{eff}} = \frac{1}{3} \left( \tau_{\text{DP},s_{x+}} + \tau_{\text{DP},s_{x-}} + \tau_{\text{DP},s_z} \right). \quad (\text{S24})$$

Here we average the spin relaxation times rather than the spin relaxation rates. This is because we have three independent, equally populated spin components that are each relaxing through its own, separate channels (diffusion), in contrast to a single spin species that can relax through three different channels. More precisely, we note that the initial electron spin in a loop can point (with equal probabilities) along the  $s_{x-}$ ,  $s_{x+}$ , and  $s_z$  axes (analogous to  $x_+$ ,  $x_-$ , and  $z$ , respectively), which have unequal (and independent) spin-dephasing times  $\tau_{\text{DP},s_{x-}}$ ,  $\tau_{\text{DP},s_{x+}}$ , and  $\tau_{\text{DP},s_z}$ . Hence we take  $\tau_{\text{eff}}$  to be the average in Eq. S24. Note that this also correctly results in a diverging  $\tau_{\text{eff}}$  for  $\alpha = \pm\beta$  in case of negligible  $\beta_3$ . With this at hand, we can define an effective diffusive SO length  $\lambda_{\text{eff}} = \sqrt{2D\tau_{\text{eff}}}$  reading

$$\lambda_{\text{eff}} = \frac{\hbar^2}{\sqrt{6}m^*} \sqrt{\left[ (\alpha - \beta)^2 + \frac{\tau_3}{\tau_1} \beta_3^2 \right]^{-1} + \left[ (\alpha + \beta)^2 + \frac{\tau_3}{\tau_1} \beta_3^2 \right]^{-1} + \frac{1}{2} \left[ \alpha^2 + \beta^2 + \frac{\tau_3}{\tau_1} \beta_3^2 \right]^{-1}} \quad (\text{S25})$$

Equivalently, this average spin diffusion length can be defined from the variance  $\bar{\sigma}_{x_i}^2 = (\sigma_{x_i,s_{x-}}^2 + \sigma_{x_i,s_{x+}}^2 + \sigma_{x_i,s_z}^2)/3$ , along  $\hat{x}_i$   $i = +, -$ , obtained by averaging over the initial spin directions. At  $\alpha = \pm\beta$  and small  $\beta_3$  (and/or  $\tau_3 \ll \tau_1$ ) the SO length  $\lambda_{\text{eff}}$  diverges, as explained in the main text. We fit our data points using Eq. S25 and the ratio  $\tau_3/\tau_1$  as a free parameter, as shown in Fig. S9. The resulting ratio  $\tau_3/\tau_1 \lesssim 0.2$  (0.4) for  $n = 6 \cdot 10^{11} \text{ cm}^{-2}$  ( $9 \cdot 10^{11} \text{ cm}^{-2}$ ) can be explained by small angle scattering, originating from the long range potential of the remote donors.

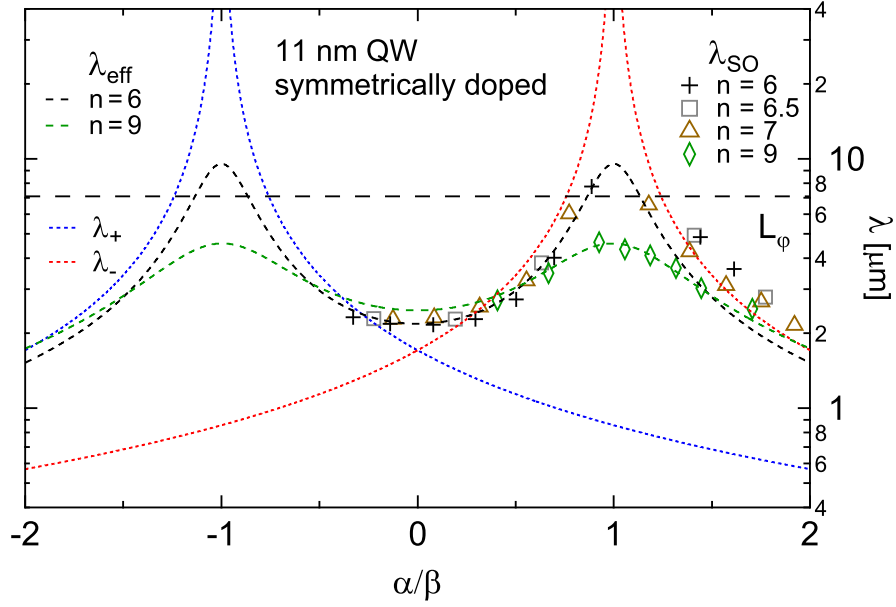

FIG. S9. Theoretical and experimental SO lengths including symmetry breaking. In contrast to the ballistic  $\lambda_{\pm}$  (dotted red and blue), the diffusive  $\lambda_{\text{eff}}$  (dashed black and green, fits to  $\lambda_{\text{SO}}$  data points) includes the symmetry breaking higher harmonic term and does not diverge at  $\alpha = \pm\beta$ . The highest density  $n = 9 \cdot 10^{11} \text{ cm}^{-2}$  (green markers) shows the strongest symmetry breaking effect, where WAL remains visible through  $\alpha = \pm\beta$ , thus allowing extraction of  $\lambda_{\text{SO}} < L_{\varphi}$  at  $\alpha = \beta$ .

### C. Equivalence between ballistic and spin-diffusion lengths

We now argue that the ballistic spin precession lengths  $\lambda_{\pm} = \hbar^2/(2m^*|\alpha \pm \beta|)$  introduced in the main text and the spin diffusion lengths  $\lambda_{s_{x-}}^{\text{DP}} = \sqrt{\sigma_{s_{x-}}^2} = \sqrt{2D\tau_{\text{DP},s_{x-}}}$  and  $\lambda_{s_{x+}}^{\text{DP}} = \sqrt{\sigma_{s_{x+}}^2} = \sqrt{2D\tau_{\text{DP},s_{x+}}}$  defined via the DP random-walk process are equivalent. Here we drop the index  $x_i$  on the variance, as it does not depend on  $\hat{x}_i$  since  $D$  is assumed isotropic in our model (Sec. V A), and add a spin index to it, which we had mostly omitted in the preceding paragraphs for ease of notation. From its definition,  $\lambda_{s_{x-}}^{\text{DP}}$  describes the spin diffusion length for an electron performing a random walk in two dimensions with its spin pointing initially along  $s_{x-}$ . A similar interpretation holds for  $\lambda_{s_{x+}}^{\text{DP}}$ . The definition of the ballistic  $\lambda_{\pm}$  did not include third harmonic effects. Thus when setting to zero the third harmonic term in Eq. S22 and converting the resulting  $\tau_{\text{DP},s_{x\pm}}$  to lengths using  $\lambda_{s_{x+}}^{\text{DP}}$  and  $\lambda_{s_{x-}}^{\text{DP}}$ , we obtain straightforwardly  $\lambda_{s_{x+}}^{\text{DP}} = \hbar^2/(\sqrt{2}m^*|\alpha + \beta|) \simeq \lambda_+$  and  $\lambda_{s_{x-}}^{\text{DP}} = \hbar^2/(\sqrt{2}m^*|\alpha - \beta|) \simeq \lambda_-$ . The diffusion constant  $D$  cancels in the conversion from time to length. Hence the diffusive spin relaxation length and the ballistic spin precession length are mathematically equivalent.

The physical reason for this equivalence is as follows. Firstly, recall that the ballistic precession lengths  $\lambda_{\pm}$  define distances over which an electron traveling along  $\hat{x}_{\pm}$  with its spin perpendicular to the effective Rashba-Dresselhaus field [Eq. S20] precesses by 1 radian. More specifically, an electron traveling along  $\hat{x}_{-}$  ( $\hat{x}_{+}$ ) with its spin pointing along either  $\hat{x}_{-}$  ( $\hat{x}_{+}$ ) or  $\hat{z}$  (or any linear combination of these) will undergo spin precession about  $\mathbf{B}_{\text{RD}}^{(1)}(k_{-}, 0) = \frac{2}{g\mu_B}(\beta - \alpha)k_{-}\hat{x}_{+}$  ( $\mathbf{B}_{\text{RD}}^{(1)}(0, k_{+}) = \frac{2}{g\mu_B}(\beta + \alpha)k_{+}\hat{x}_{-}$ ) covering a distance  $\lambda_{-}$  ( $\lambda_{+}$ ) as it rotates by 1 radian. Secondly, note that the spin diffusion length  $\lambda_{s_{x_{-}}}^{\text{DP}}$  ( $\lambda_{s_{x_{+}}}^{\text{DP}}$ ) denotes a distance over which an electron moving initially along an *arbitrary* direction on the  $(x_{+}, x_{-})$  plane and with its spin pointing along  $s_{x_{-}}$  ( $s_{x_{+}}$ ), accrues a net precession of 1 radian about the total Rashba-Dresselhaus field [Eq. S20] after many random momentum scattering events. However, because the initial spin polarization is pointing along  $s_{x_{-}}$  ( $s_{x_{+}}$ ) we can neglect the Rashba-Dresselhaus field component that is parallel to  $s_{x_{-}}$  ( $s_{x_{+}}$ ), i.e., the  $\hat{x}_{-}$  ( $\hat{x}_{+}$ ) component, when calculating the spin dephasing due to the DP mechanism. This is physically justified as the precession around the parallel field component does not drive the spin direction away from its initial spin polarization, but rather just randomizes its phase around that direction. In the presence of just the  $x_{+}$  ( $x_{-}$ ) component of  $\mathbf{B}_{\text{RD}}$ , which is perpendicular to the initial  $s_{x_{-}}$  ( $s_{x_{+}}$ ), the real-space random-walk problem in two dimensions becomes a 1D problem in spin space with the electron spin performing random (“Abelian”) precessions about this unidirectional field component. What we just described, despite 2D charge diffusion, is similar to a ballistic spin precession about a fixed axis, which is precisely what  $\lambda_{+}$  ( $\lambda_{-}$ ) is; hence the equivalence between the spin diffusion  $\lambda_{s_{x_{-}}}^{\text{DP}}$  ( $\lambda_{s_{x_{+}}}^{\text{DP}}$ ) and ballistic  $\lambda_{+}$  ( $\lambda_{-}$ ) lengths. Note that when the initial spin polarization for the diffusive motion is pointing along  $s_z$  then both components of the Rashba-Dresselhaus field are relevant for spin dephasing away from this initial spin direction; a simple calculation using  $\lambda_{s_z}^{\text{DP}} = \sqrt{2D\tau_{\text{DP}, s_z}}$  and Eq. S23 yields  $\lambda_{s_z}^{\text{DP}} = \hbar^2 / (2m^* \sqrt{\alpha^2 + \beta^2})$ .

## VI. SHUBNIKOV-DE HAAS OSCILLATIONS

In this section we show Shubnikov-de Haas (SdH) oscillations measured during a separate cooldown of the 9.3 nm wafer. Measurements were performed in a dilution refrigerator with base temperature 20 mK. We have used a standard four-wire lock-in technique at 633 Hz and 100 nA current bias. In Fig. S10 a) and b) the density and mobility maps for this

cooldown are shown. The lower panels labeled with 1-3 show the SdH oscillations (left column) and their respective Fourier spectra (right column) for a contour of constant density ( $n = 4.5 \cdot 10^{11} \text{ cm}^{-2}$ ) as indicated in the density and mobility map. In Fig.S11 the SdH oscillations and Fourier spectra for the gate configurations 4-6 from Fig.S10 a) are shown.

The SdH oscillations are clearly visible for all gate configurations. In the Fourier spectra we see a peak at the fundamental frequency of approximately 10 cycles per Tesla and multiples of it. Panel 1 of Fig.S10 also shows the SdH oscillations calculated from theory (to be presented elsewhere) with up to  $k = 6$  Fourier components (black). These higher harmonics are clearly seen in the Fourier spectra and are in good agreement with the experimentally observed ones. We also note that these peaks are not accompanied by any additional peaks. The influence of the SO interaction on the magnetoconductance oscillations can cause a spin splitting of the subbands which leads to a beating pattern in the oscillations. Here we do not see any beating nor are there any other frequencies visible. The beating pattern due to SO induced spin splitting has been reported in  $\text{In}_x\text{Ga}_{1-x}\text{As}$  quantum wells [16]. Generally the SO strength is much larger in In-based semiconductors than in GaAs, thus one would not expect to see here a beating of the SdH oscillations. We try to estimate the beating frequency compared to the SdH frequency for the measured data. The MC oscillations can simply be described by an oscillation of the density of states in  $1/B$  [8]. For a beating to occur there must be two frequencies. By comparing the relevant energy scales we can get an estimate about the period with which the beating would occur in the low field regime. For simplicity we assume only a contribution of the Rashba SO interaction. We compare the Fermi energy  $E_F$  to the Rashba energy  $E_R = \alpha k_F$ . We get  $E_R = 2\alpha k_F = 0.13 \text{ meV}$  and  $E_F = \frac{\hbar^2 k_F^2}{2m^*} = 14.0 \text{ meV}$ , where we have used  $\alpha \approx 8 \text{ meV}\text{\AA}$  and  $n = 4.5 \cdot 10^{11} \text{ cm}^{-2}$ . This means that these beatings would occur at a very large magnetic field, which is beyond the low field limit. Thus it is impossible to observe these oscillations in our data.

- 
- [1] K. D. Maranowski, J. P. Ibbetson, K. L. Campman, and A. C. Gossard, *Applied Physics Letters* **66**, 3459 (1995).
  - [2] R. S. Calsaverini, E. Bernardes, J. C. Egues, and D. Loss, *Physical Review B* **78**, 155313 (2008).

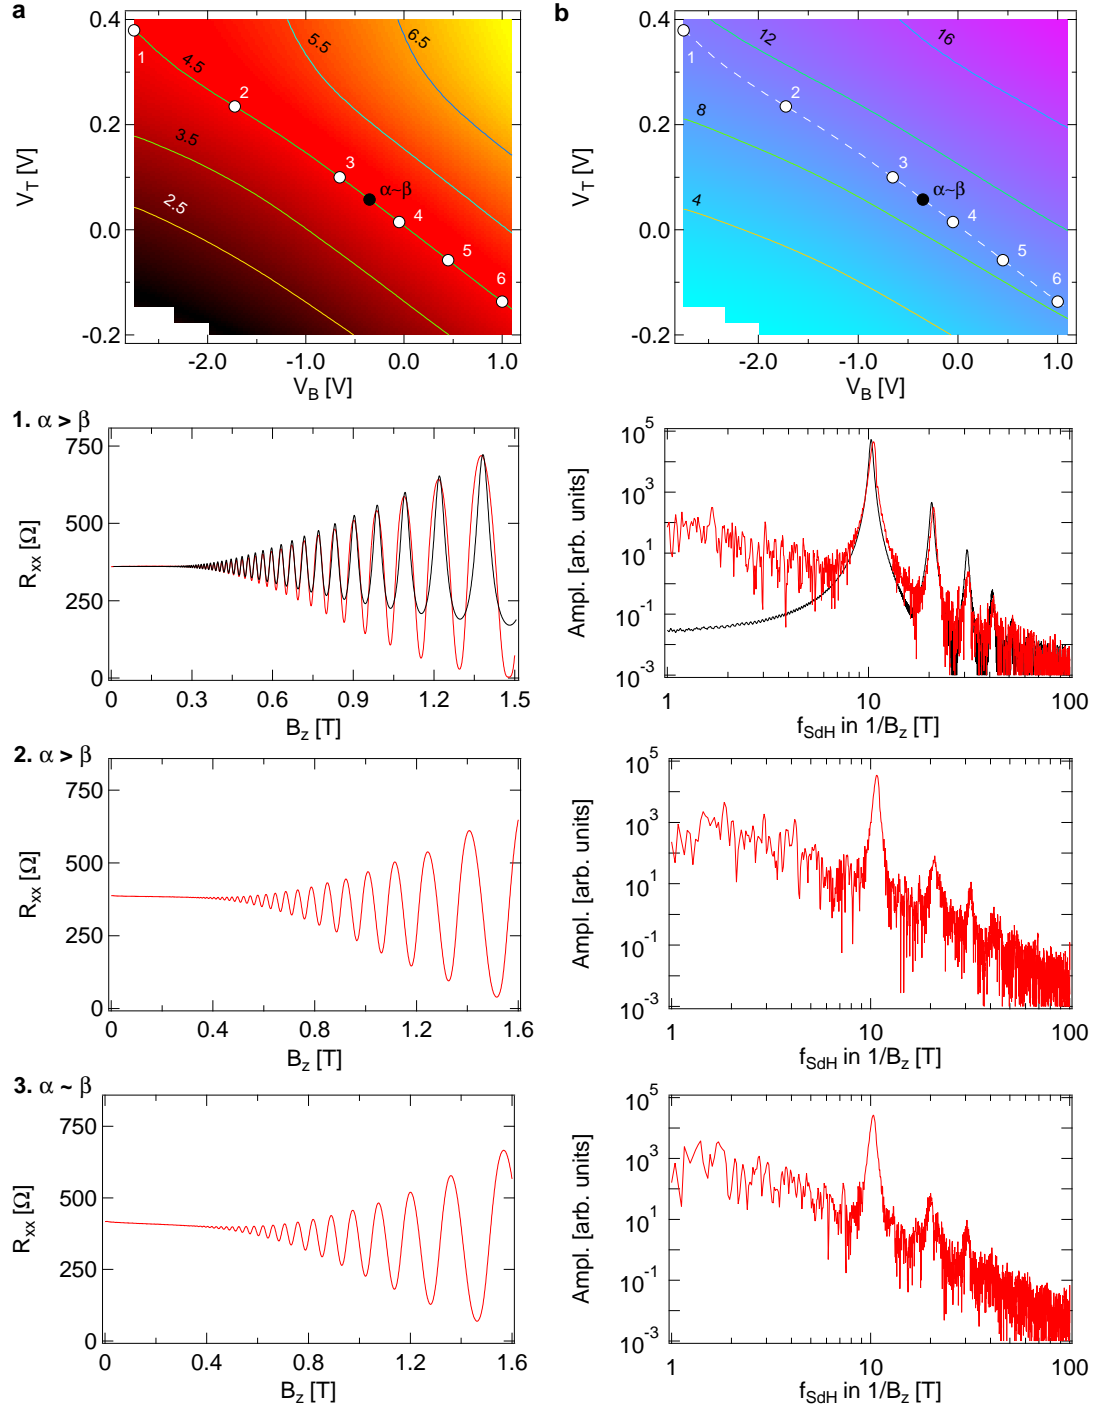

FIG. S10. Shubnikov de Haas oscillations measured on the 9.3 nm QW - I. Charge carrier density  $n$  (a) and mobility (b) as a function of top gate voltage  $V_T$  and back gate voltage  $V_B$ . Contour lines are labeled in units of  $10^{11} \text{ cm}^{-2}$  (a) and  $\text{m}^2/\text{Vs}$  (b), respectively. Gate configurations at which the SdH data was measured are indicated on the density and mobility map as points labeled with 1-6. The gate configuration at which  $\alpha = \beta$  is also shown. In the panel below the corresponding SdH oscillations at the gate configurations 1-3 are shown (left column) and beside its Fourier spectra (right column). In panel 1 the SdH oscillations plotted from theory and its Fourier spectrum are shown as well (black curves).

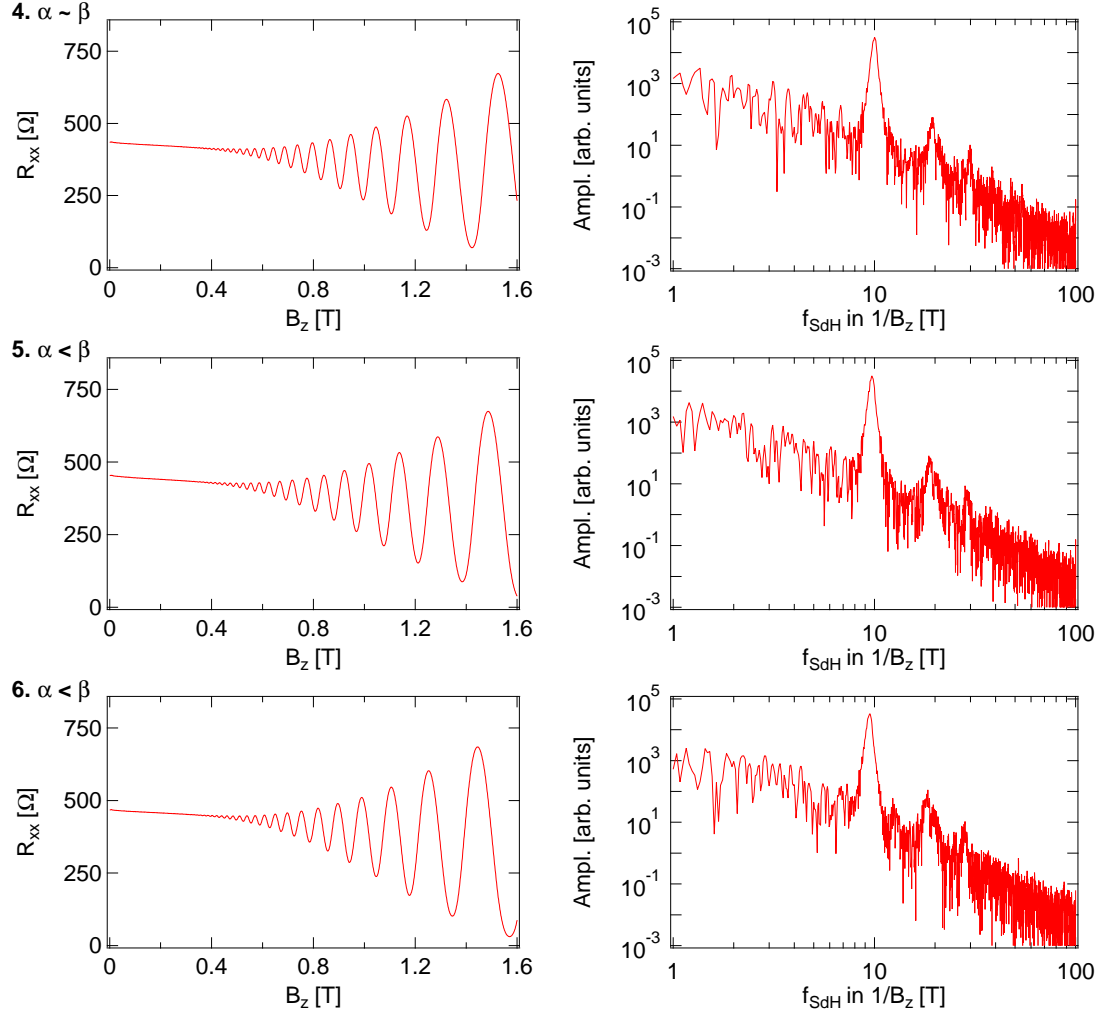

FIG. S11. Shubnikov-de Haas oscillations measured on the 9.3 nm QW - II. Continued SdH oscillations and their Fourier spectra for the gate configurations 4-6 as indicated in Fig. S10 a.

- [3] G. Dresselhaus, *Physical Review* **100**, 580 (1955).
- [4] J.-M. Jancu, R. Scholz, E. de Andrada e Silva, and G. La Rocca, *Physical Review B* **72** (2005), 10.1103/PhysRevB.72.193201.
- [5] W. Yi, V. Narayanamurti, H. Lu, M. A. Scarpulla, A. C. Gossard, Y. Huang, J. H. Ryou, and R. D. Dupuis, *Applied Physics Letters* **95**, 112102 (2009).
- [6] I. Vurgaftman, J. R. Meyer, and L. R. Ram-Mohan, *Journal of Applied Physics* **89**, 5815 (2001).
- [7] H. Mayer and U. Rössler, *Physical Review B* **44**, 9048 (1991).
- [8] R. Winkler, *Spin-orbit coupling effects in two-dimensional electron and hole systems* (Springer, Berlin and New York, 2003).

- [9] The split-off hole offset is written as,  $\delta_{\Delta} = \Delta_b + \delta_v - \Delta_w$ . Based on the parameters listed in Table I, we have,  $\delta_{\Delta} = (0.3287 \pm 0.006) \text{ eV} + (0.171 \pm 0.003) \text{ eV} - (0.341 \pm 0.001) \text{ eV} = (0.1587 \pm 0.01) \text{ eV}$ .
- [10] C. Hermann and C. Weisbuch, *Physical Review B* **15**, 823 (1977).
- [11] M. Cardona, N. E. Christensen, and G. Fasol, *Physical Review B* **38**, 1806 (1988).
- [12] S. V. Iordanskii, Y. B. Lyanda-Geller, and G. E. Pikus, *JETP Letters* **60**, 206 (1994).
- [13] M. M. Glazov and L. E. Golub, *Semiconductor Science and Technology* **24**, 064007 (2009).
- [14] F. Reif, *Fundamentals of Statistical and Thermal Physics* (McGraw Hill, Tokyo, 1965).
- [15] N. S. Averkiev, L. E. Golub, and M. Willander, *Journal of Physics: Condensed Matter* **14**, R271 (2002).
- [16] B. Das, D. C. Miller, S. Datta, R. Reifenberger, W. P. Hong, P. K. Bhattacharya, J. Singh, and M. Jaffe, *Physical Review B* **39**, 1411 (1989).
